# Supplementary material for: Composing Diverse Policies for Temporally Extended Tasks
Source: arXiv:1907.08199 source file (2020-02-17)
Supplement: Supplementary file 1 [file 9-supplementary_material.tex]

\section*{Supplementary Material}

This material includes additional detail around the controller components used for experimentation. For obtaining the neural policies (e.g. Figure.\ref{fig:gear_peg}) we used the following rule of thumb:

\begin{itemize}
    \item We use a Behaviour Cloning loss with the VAE loss to train our policy models with Adam with $\alpha = 0.001$ with weight decay of $1e^{-6}$. We obtained 50 demonstrations of each subtask.

    \item Our input image has a size of $128x128$ pixels. We observe that the Neural Network Policy does not require a sophisticated feature extractor like ResNet50, ResNet101 to create necessary features for the task. Using those extractors leads to the same final performance, but increases the training time significantly. We use 5 convolutional layers of 4x4 filters with batch normalization and leaky ReLUs.

    \begin{table}[h]
        \centering
        \begin{tabular}{lcc}
        \hline
                   & Sub Task Performance & Full Task Performance \\ \hline
        ResNet50   & 10/10                & 10/10                 \\
        ResNet101  & 10/10                & 10/10                 \\
        Small Conv & 10/10                & 10/10                
        \end{tabular}
    \end{table}
    
    \item Additional ``what-if'' \textit{(it's tilted, flipped, not visible, etc.)} training examples were detrimental to the performance of the model. In order to incorporate that part of the state space, a full set of overlapping and interpolating examples need to be provided.
\end{itemize}

\begin{figure*}
\centering
\includegraphics[width=1.\linewidth]{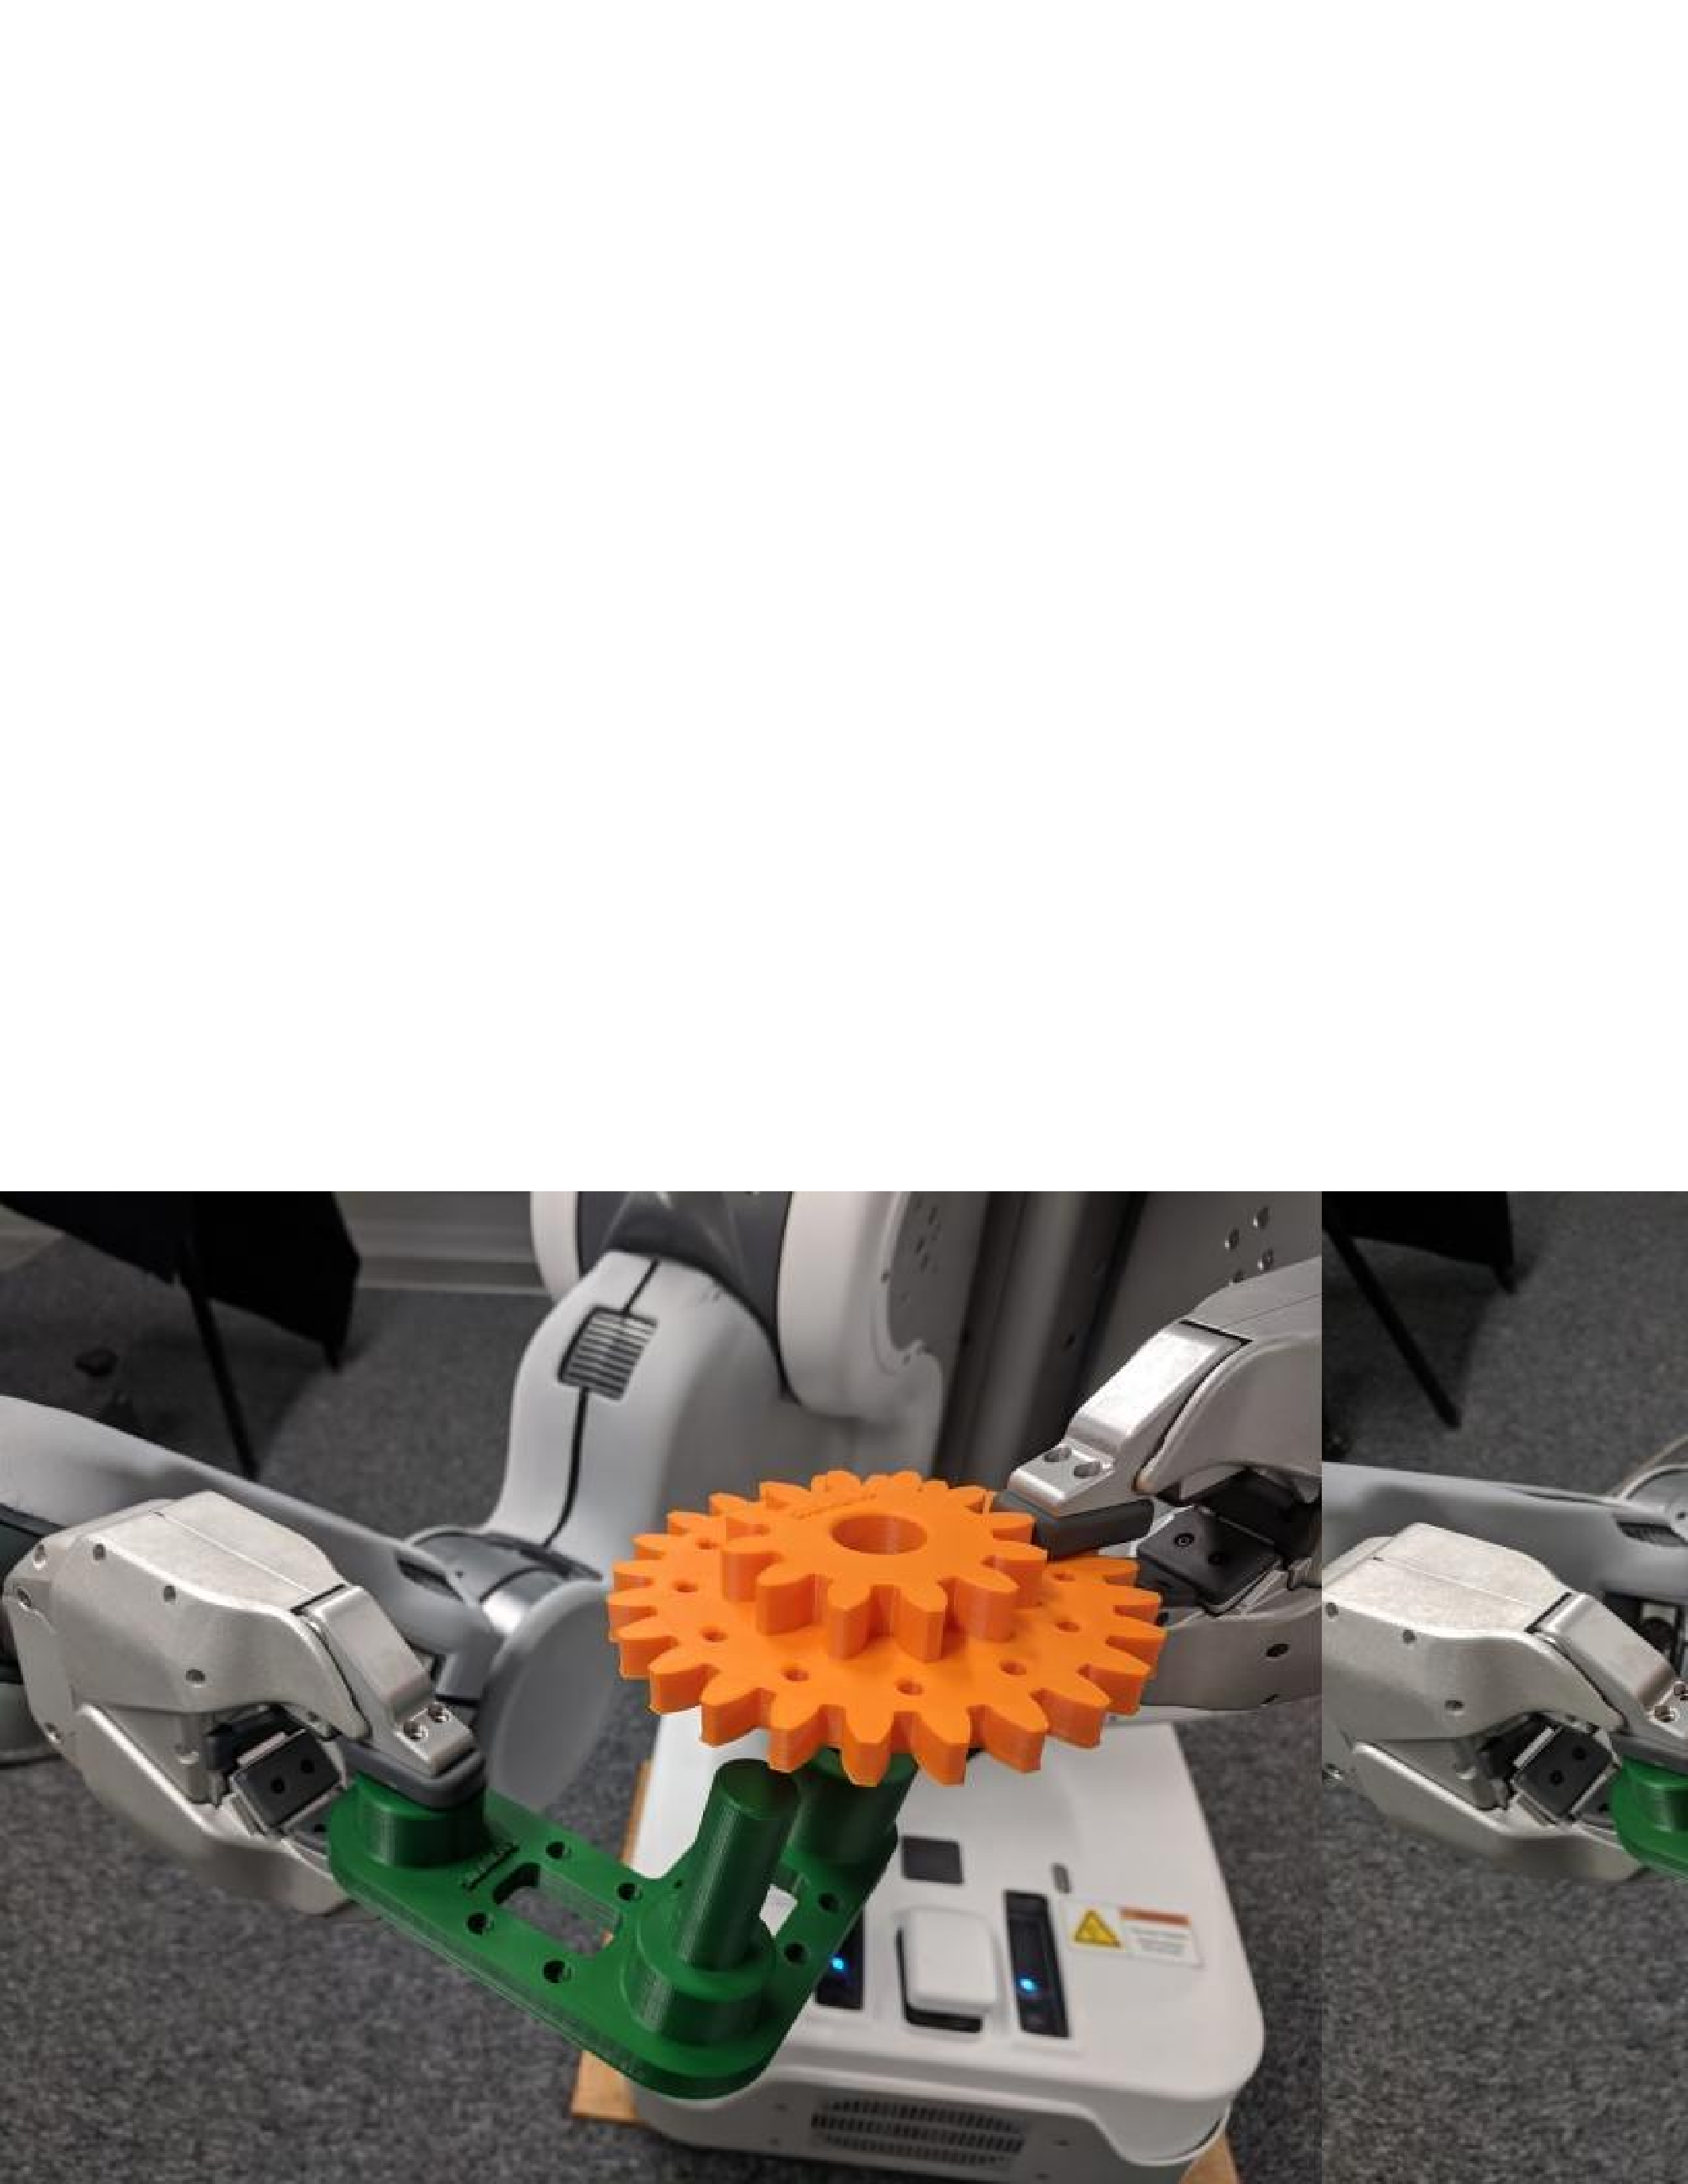}
\caption{The execution of a neural network policy for inserting the gear on the peg. }
\label{fig:gear_peg}
\end{figure*}
